# Supplementary material for: Efficient Dataset Distillation via Minimax Diffusion
Source: arXiv:2311.15529 source file (2024-03-25)
Supplement: Supplementary file 1 [file appendix.tex]

\section{Visualization of Generated Images}

\section{Extended Related Works}
